# Supplementary material for: Panoptic-aware Image-to-Image Translation
Source: arXiv:2112.01926 source file (2022-12-22)
Supplement: Supplementary file 1 [file supplimentary.tex]

\documentclass[10pt,twocolumn,letterpaper]{article}

\usepackage{wacv}
\usepackage{times}
\usepackage{epsfig}
\usepackage{graphicx}
\usepackage{amsmath}
\usepackage{amssymb}
\usepackage{booktabs}
\graphicspath{./images/}
\usepackage{float}
\usepackage[caption=false,font=normalsize,labelfont=sf,textfont=sf]{subfig}
\usepackage{cite}
\usepackage{multirow}
\usepackage[accsupp]{axessibility}  % Improves PDF readability for those with disabilities.
% Include other packages here, before hyperref.

%%%%%%%%%%%%%%%%%%%%%%%%%%%%%%%%%%%%%%%%%%%%%%%%%%%%%%%%%%%%%%%%%%%%%%%%%%%%%%%%
%
%%% IMPORTANT - These next three lines are CRUCIAL.
%               (1) PLEASE enter your paper ID (given by CMT) replacing the
%                   '****' right below here with the ID from CMT.
%               (2) If you are submitting to the Algorithms track, then uncomment
%                   the \wacvalgorithmstrack line below. If you are submitting to the
%                   Applications track, then uncomment the \wacvapplicationstrack line.
%                   If you do not update this properly, we cannot guarantee
%                   that your paper will be evaluated according to the correct
%                   review criteria!
%               (3) Leave the \wacvfinalcopy commented out for the submission
%                   version, but UNCOMMENT it for your CAMERA-READY upload.
 
%(1)
 % Enter the WACV Paper ID here

%(2)
\wacvalgorithmstrack   % Uncomment this line if you are submitting to the Algorithms Track.
%\wacvapplicationstrack % Uncomment this line if you are submitting to the Applications Track.

%(3)
\wacvfinalcopy % *** Uncomment this line for the final submission

%%%%%%%%%%%%%%%%%%%%%%%%%%%%%%%%%%%%%%%%%%%%%%%%%%%%%%%%%%%%%%%%%%%%%%%%%%%%%%%%

% If you comment hyperref and then uncomment it, you should delete
% egpaper.aux before re-running latex.  (Or just hit 'q' on the first latex
% run, let it finish, and you should be clear).
\ifwacvfinal
\usepackage[breaklinks=true,bookmarks=false]{hyperref}
\else
\usepackage[pagebackref=true,breaklinks=true,colorlinks,bookmarks=false]{hyperref}
\fi

% Pages are numbered in submission mode, and unnumbered in camera-ready
% \pagestyle{empty}
\setcounter{page}{1}

\begin{document}

%%%%%%%%% TITLE
\title{Panoptic-aware Image-to-Image Translation\\
Supplementary Material}

\author{Liyun Zhang$^{1}$, Photchara Ratsamee$^{1,2}$, Bowen Wang$^{1}$, Zhaojie Luo$^{1}$, Yuki Uranishi$^{1}$,\\
Manabu Higashida$^{1}$ and Haruo Takemura$^{1}$\\
$^{1}$Osaka University, Japan {\tt\small liyun.zhang@lab.ime.cmc.osaka-u.ac.jp}\\
$^{2}$Osaka Institute of Technology, Japan {\tt\small photchara@ime.cmc.osaka-u.ac.jp}\\
}

\maketitle
\thispagestyle{empty}

%%%%%%%%% BODY TEXT
\section{Overview}
In this supplementary, we first describe the cLSTM \cite{cLSTM} component of our model in Section \ref{sec:clstm}.
The detailed setting of evaluation metrics is described in Section \ref{sec:metrics}.
We also show the description of our contributed dataset in Section \ref{sec:dataset}.
In Section \ref{sec:efficiency}, we provide the discussion of model efficiency.
We show the additional experimental results in Section \ref{sec:examples}.
Also, the limitation discussion is provided in Section \ref{sec:limitations}.
%-------------------------------------------------------------------------

\section{cLSTM \cite{cLSTM} component}
\label{sec:clstm}
After feature masking, the masked object feature maps need to be fused into a well-hidden representation for generating a realistic target image.
Therefore, we need to integrate all objects in the desired locations and coordinate object feature maps based on other objects in the image.
As shown in Fig.~\ref{CLSTM}, the convolutional Long-Short-Term Memory (cLSTM) \cite{cLSTM} is a multi-layer convolutional LSTM network, where the hidden states and cell states are both feature maps rather than vectors different from the traditional LSTM \cite{LSTM}.
The computation of different gates is also done by convolutional layers.
Therefore, cLSTM can better preserve spatial information compared with the traditional vector-based LSTM.
It can integrate each object feature maps $\left\{F_{{obj}_i}\right\}_{i=1}^{m}$ one-by-one along the object sequence of $1 \sim m$ obtained by panoptic perception.
The last output of cLSTM is used as the fused hidden representation $H_{obj}$.
Different objects are sequentially fused together while keeping their spatial locations in the image.

\begin{figure}[ht]
\begin{center}
\includegraphics[width=1.0\linewidth]{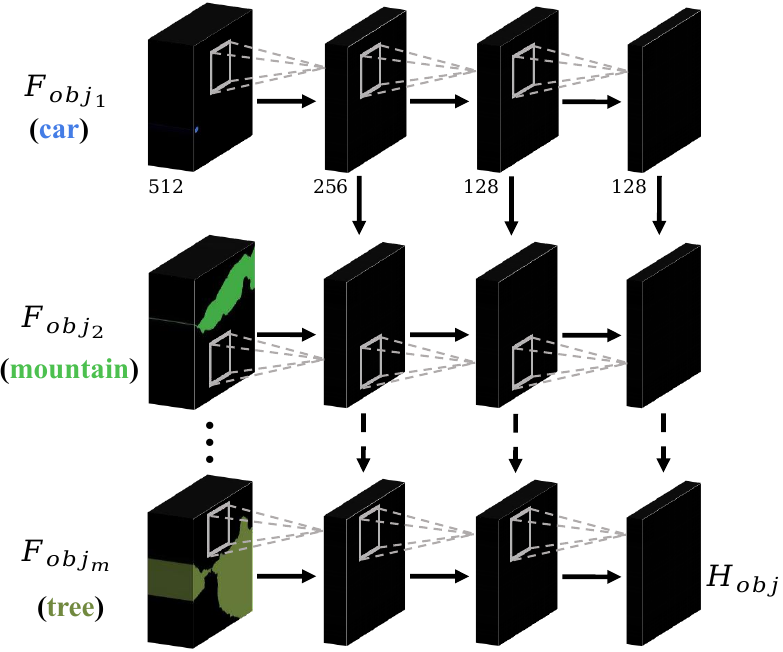}
\end{center}
    \caption{Illustration of convolutional Long-Short-Term Memory (cLSTM) component. We use three layers cLSTM for fusing all object feature maps together into the hidden feature maps $H_{obj}$. The number of channels in each layer of cLSTM is 256, 128, 128, respectively. The residual blocks are omitted for clarity. The first of each row is object feature maps of $F_{obj} = \left\{F_{{obj}_i}\right\}_{i=1}^{m}$.}
\label{CLSTM}
\end{figure}
%-------------------------------------------------------------------------

\section{Evaluation metrics}
\label{sec:metrics}
We chose the Human Preference (HP), Inception Score (IS) \cite{IS}, Fréchet Inception Distance (FID) \cite{FID_KID} and Diversity Score (DS) metrics instead of Peak Signal-to-Noise Ratio (PSNR) and Structure Similarity Index (SSIM) \cite{SSIM} metrics to evaluate the image quality.
Because for images generated by GANs learning models, traditional PSNR and SSIM metrics deviate from human visual perception \cite{LPIPS}.
Also, we chose Panoptic Quality (PQ) \cite{Panoptic-Segmentation} series metrics instead of instance segmentation and object detection to evaluate object recognition performance.
Because PQ series metrics combine mean Intersection over Union (mIoU) in segmentation quality (SQ) and average precision (AP) in recognition quality (RQ) for more comprehensive scores.
Also, since our framework is based on panoptic perception, using PQ series metrics will be more appropriate than the traditional object recognition metrics.

{\bf Human Preference (HP)} compares the image quality through human cognition.
We divided each evaluation set results into 5 groups to show to 5 persons in 20 participants (average age: 29.90, std: 23.49) in turn.
Each group's images are selected with the best three results corresponding to realism, object sharpness and scene similarity respectively with unbiased weights (1:1:1) to ensure adequate fairness of evaluation.
The total number of selections is calculated as a final comprehensive percentage score.

{\bf Inception Score (IS) \cite{IS}} uses an Inception V3 network pre-trained on the ImageNet-1000 classification benchmark and computes a statistics score of the network’s outputs \cite{LOST-GAN2}.
The higher the IS is, the better a generator model is.

{\bf Fréchet Inception Distance (FID) \cite{FID_KID}} also uses an Inception V3 network pre-trained on the ImageNet like IS to compute the Frèchet distance \cite{FID} between two Gaussian distributions fitted to synthesized images and real images respectively \cite{LOST-GAN2}.
The lower the FID is, the better a generator model is.

{\bf Diversity Score (DS)} measures the differences between paired images generated from the same input by computing the perceptual similarity in deep feature space \cite{Layout2IM}.
We used the LPIPS metric \cite{LPIPS} for diversity scoring and pre-trained AlexNet \cite{Alexnet} for feature extraction.

{\bf Panoptic Quality (PQ)} is adopted to evaluate object recognition performance, PQ combines segmentation quality (SQ) and recognition quality (RQ) \cite{Panoptic-Segmentation},

\begin{small}
\begin{equation}
\begin{aligned}
\text{PQ} = \underbrace{\begin{matrix} \dfrac{\sum_{(p,g)\in TP} \text{IoU}(p,g)}{|TP|} \end{matrix}}_{\text{segmentation \ quality (SQ)}} \times \underbrace{\dfrac{|TP|}{|TP| + \resizebox{0.015\hsize}{!}{$\dfrac{1}{2}$}|FP| + \resizebox{0.015\hsize}{!}{$\dfrac{1}{2}$}|FN|}}_{\text{recognition \ quality (RQ)}}
\end{aligned}
\end{equation}
\end{small}

where SQ sums up all of the Intersection over Union (IoU) ratios for True Positives (TP) and evaluates how closely matched predicted segments are with their ground truths.
RQ is a blend of precision and recall, where all True Positives, half False Positives (FP), and False Negatives (FN) are divided.
It combines precision and recalls to identify how effective a trained model is at getting a prediction right.
%-------------------------------------------------------------------------

\section{Dataset contribution}
\label{sec:dataset}
The unaugmented source data from our contributed dataset contains 2,026 pairs of thermal and color images based on the partial KAIST-MS \cite{KAIST-MS} dataset, it was annotated via the Segments.ai platform for the panoptic segmentation annotation by three professionally trained annotators.
The annotated datasets can be augmented by various image manipulations for a variety of different tasks.
We show the overview of annotated dataset via this link\footnote{\textbf{Overview:} https://segments.ai/panoptic/visible/}, please refer to the insights section on the overview tab to check the distribution of the categories and number of annotated objects (`thing' and `stuff').
Also, for the annotation quality and detail of images, we show the samples of the dataset on paired color images via this link\footnote{\textbf{Samples:} https://segments.ai/panoptic/visible/samples}.
%-------------------------------------------------------------------------

\section{Model efficiency}
\label{sec:efficiency}
The model efficiency will influence practical applications, it is mainly measured from computational cost, model complexity and processing time.
For the computational cost and model complexity, we used floating-point operations (FLOPs) and parameters (Params) as the evaluation indicators respectively.
For the processing time, we calculate the average processing times (Avg PT) per image for different networks of competing baselines.
As shown in Table~\ref{efficiency}, we present the model efficiency comparisons between our scores and the best baselines' scores, here we list the competing TSIT \cite{TSIT} (with +Seg, just not shown) and INIT \cite{INIT} baselines.
Table~\ref{efficiency} shows that the Params of our model are lower than other models, and FLOPs are only slightly higher than the TSIT model.
On different I2I translation tasks (summer-to-winter, day-to-night and thermal-to-color), our model spends on average less processing time than other models. 
Our method overall outperforms baselines since we use panoptic-level perception to avoid losing too much information in the translation, meanwhile, our model does not incur substantial computational cost and model complexity, also average processing time keeps competitive.

\begin{table}
    \begin{center}
        {\small{
\begin{tabular}{cccccc}
\toprule
\multirow{2}{*}{Model} & \multirow{2}{*}{Params\thinspace(M)} & \multirow{2}{*}{FLOPs\thinspace(G)} & \multicolumn{3}{c}{Avg PT\thinspace(ms)} \\
& & & $\text{t2c}$ & $\text{d2n}$ & $\text{s2w}$ \\
\midrule
TSIT & $116.1$ & $\bf{50.8}$ & $19.1$ & $19.7$ & $\bf{18.4}$ \\
INIT & $130.3$ & $62.9$ & $22.3$ & $21.0$ & $21.6$ \\
Ours & $\bf{113.6}$ & $51.4$ & $\bf{17.6}$ & $\bf{19.0}$ & $19.9$ \\
\bottomrule
\end{tabular}
}}
\end{center}
\caption{The floating-point operations (FLOPs) and parameters (Params) evaluate the computational cost and model complexity; The average processing time (Avg PT) per image evaluates processing speed. The lower the better.}
\label{efficiency}
\end{table}
%-------------------------------------------------------------------------

\section{Additional experiment results}
\label{sec:examples}
The experimental setting is the same as the main paper.
From the additional results provided in Fig.~\ref{fig:evaluation}, we further verify that most of the translation results generated by our method are better than other methods in image quality.
As illustrated in Fig.~\ref{fig:objects}, we also provide the comparison for the details of translated objects from different methods, the results demonstrate that translated objects from our method have sharper boundaries, adequate coloring, and also maintain a certain diversity, \eg, the style of cars.
Compared with competing methods on object recognition performance in Fig.~\ref{fig:perception}, our model can also obtain significant improvement.

\begin{figure*}[!t]
\captionsetup[subfloat]{labelsep=none,format=plain,labelformat=empty}
\begin{center}
\subfloat[{\bf $\text{Summer} \xrightarrow\ \text{Winter}$}]{
\includegraphics[width=1.0\linewidth]{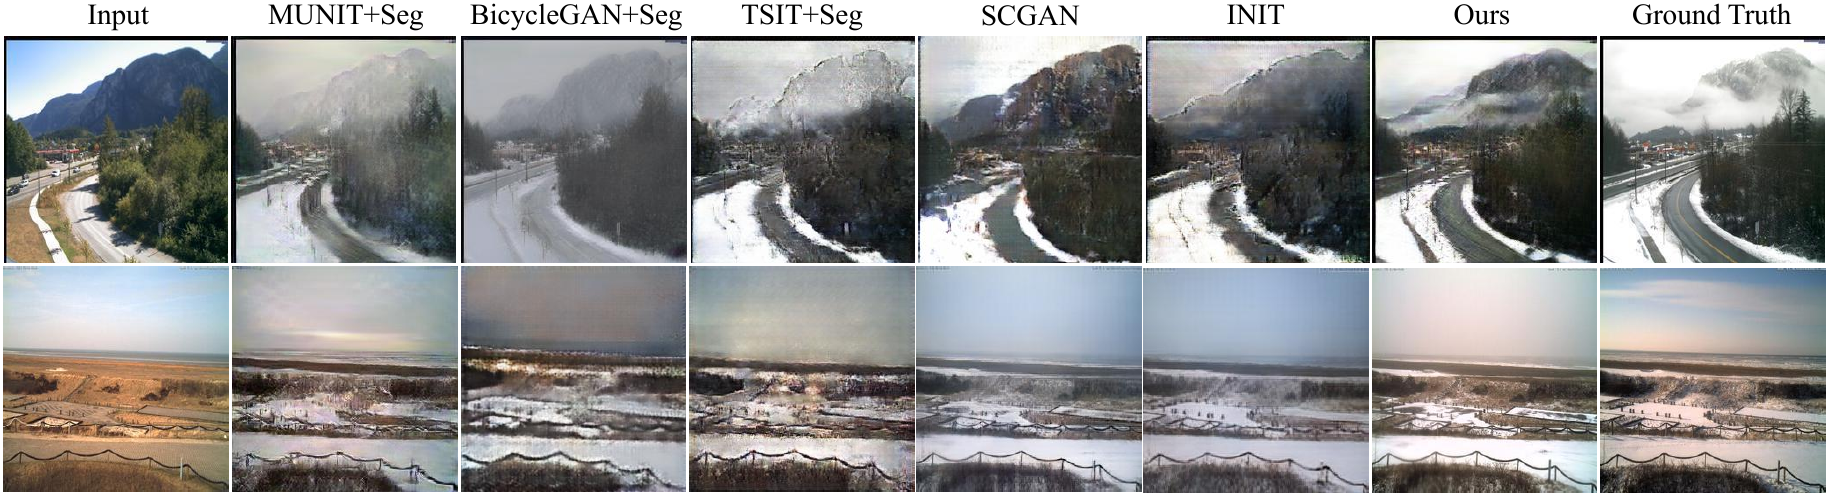}} \\
\vspace{-2.2mm}
\subfloat[{\bf $\text{Day} \xrightarrow\ \text{Night}$}]{
\includegraphics[width=1.0\linewidth]{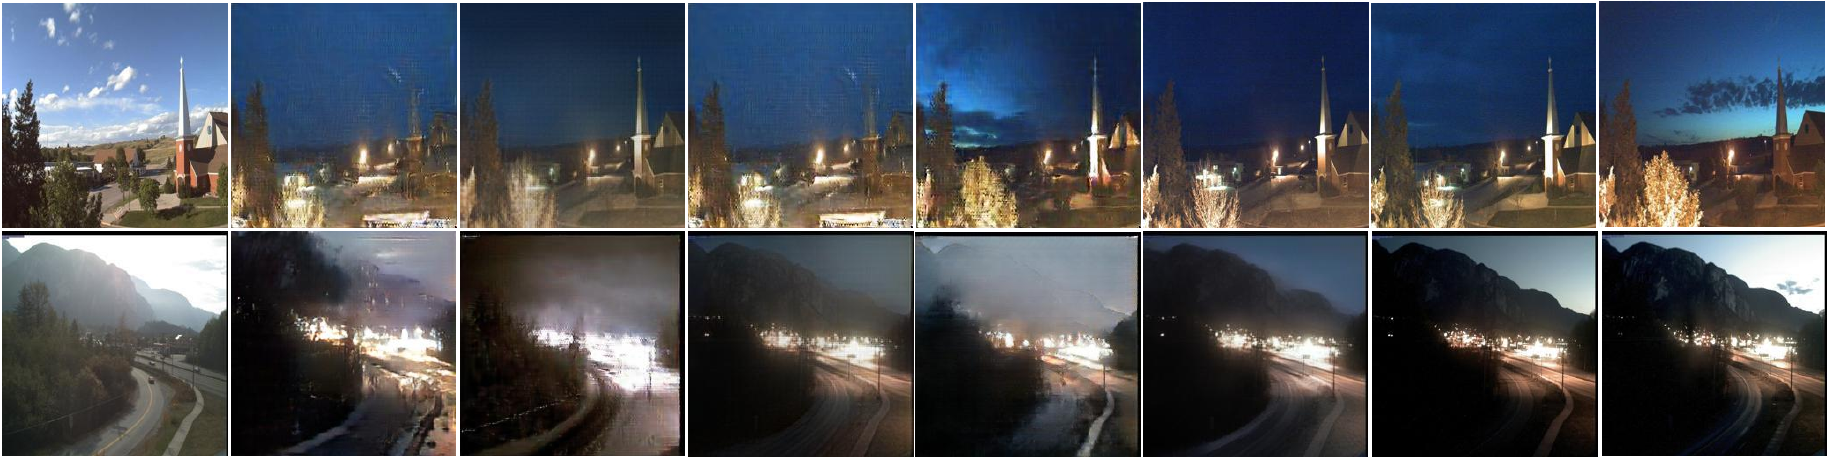}} \\
\vspace{-2.2mm}
\subfloat[{\bf $\text{Thermal} \xrightarrow\ \text{Color}$}]{
\includegraphics[width=1.0\linewidth]{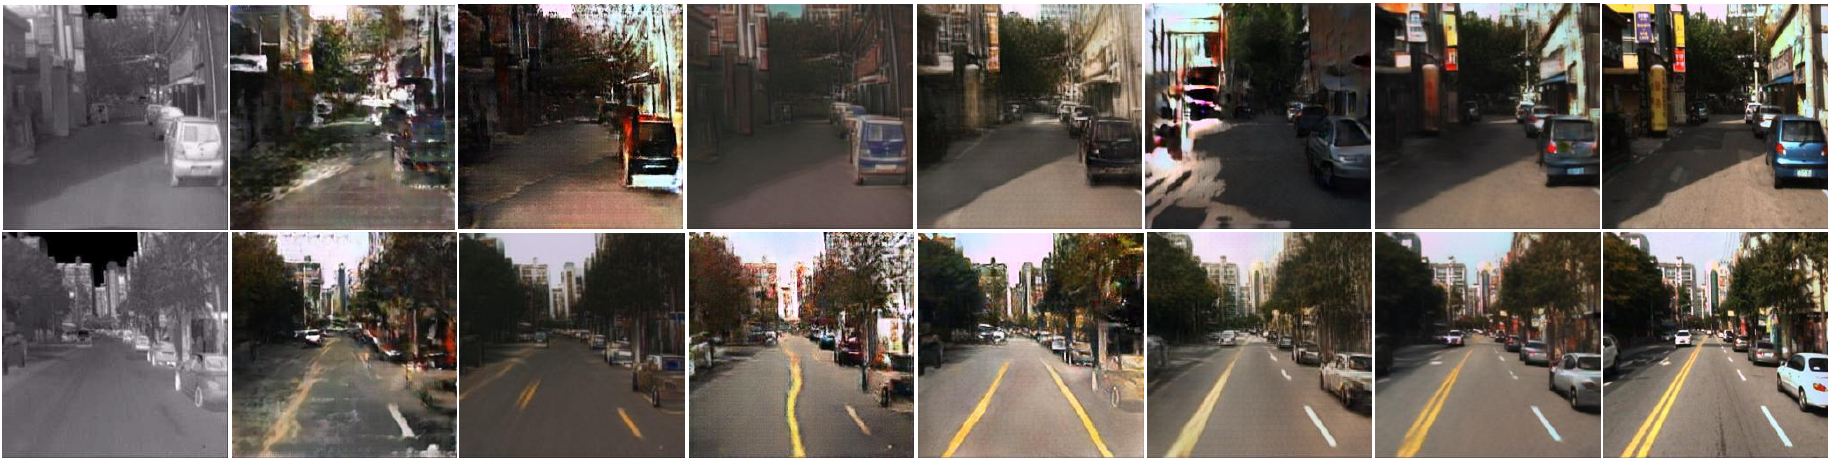}} \\
\end{center}
    \caption{Comparison of the image quality of translated images. Top group are results of the summer-to-winter I2I translation task; Middle group are results of the day-to-night I2I translation task; Bottom group are results of the thermal-to-color I2I translation task.}
\label{fig:evaluation}
\end{figure*}

\begin{figure*}[ht]
\begin{center}
\subfloat{
\includegraphics[width=1.0\linewidth]{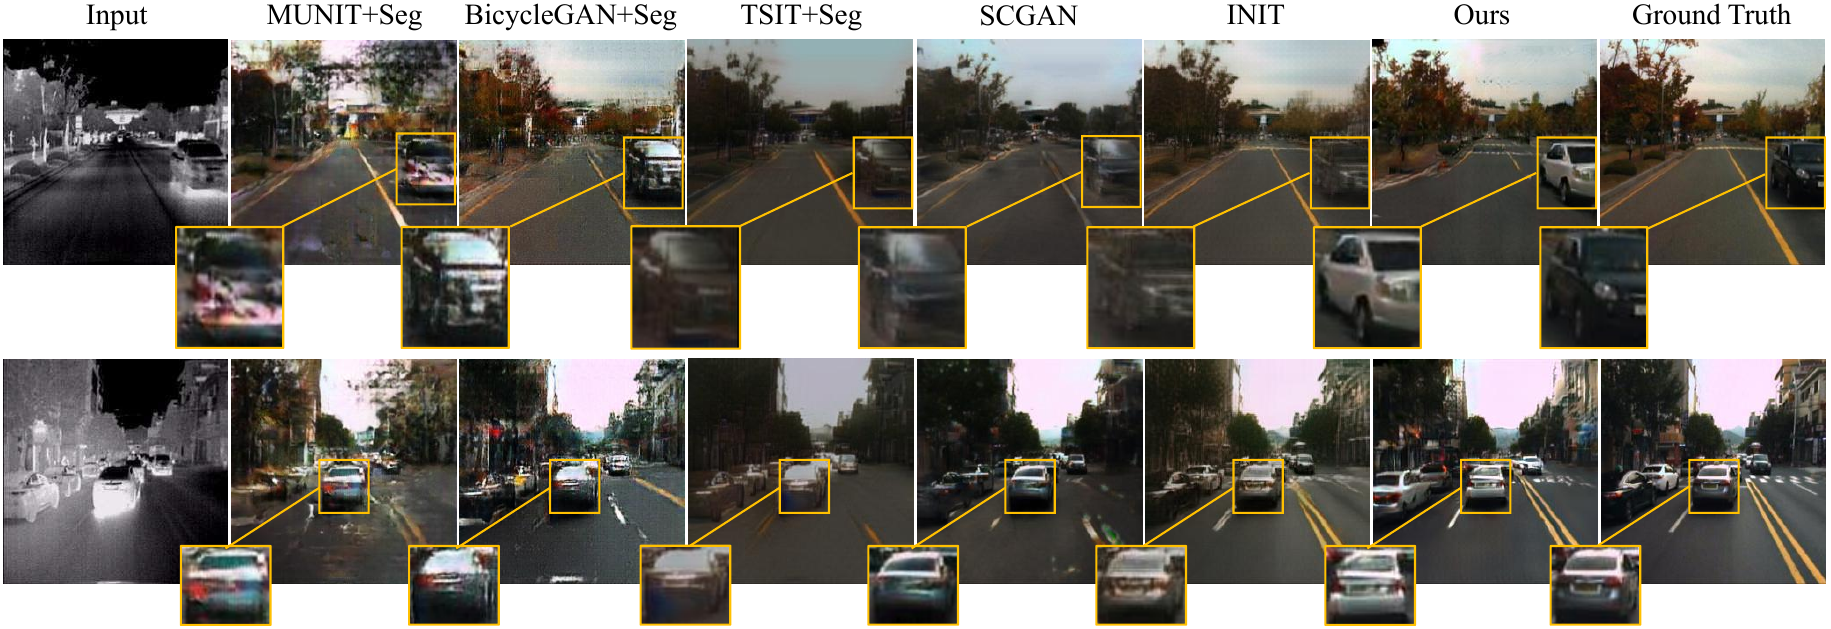}} \\
\vspace{-3.4mm}
\subfloat{
\includegraphics[width=1.0\linewidth]{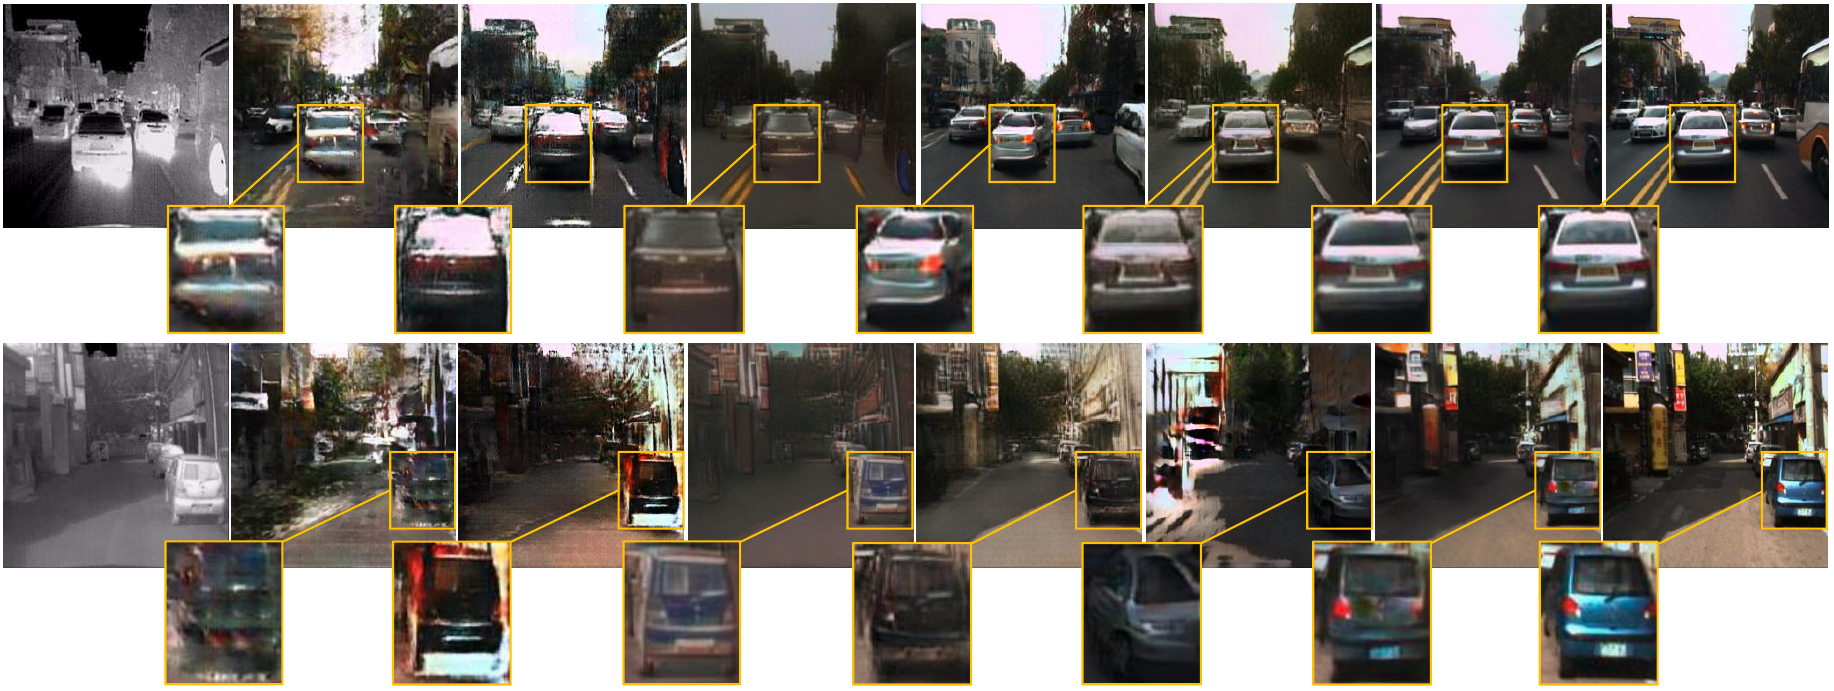}} \\
\end{center}
    \caption{Comparison results on the details of translated objects from different approaches.}
\label{fig:objects}
\end{figure*}

\begin{figure*}[ht]
\begin{center}
\captionsetup[subfloat]{labelsep=none,format=plain,labelformat=empty}
\subfloat[{\bf The scene with fewer objects}]{
\includegraphics[width=1.0\linewidth]{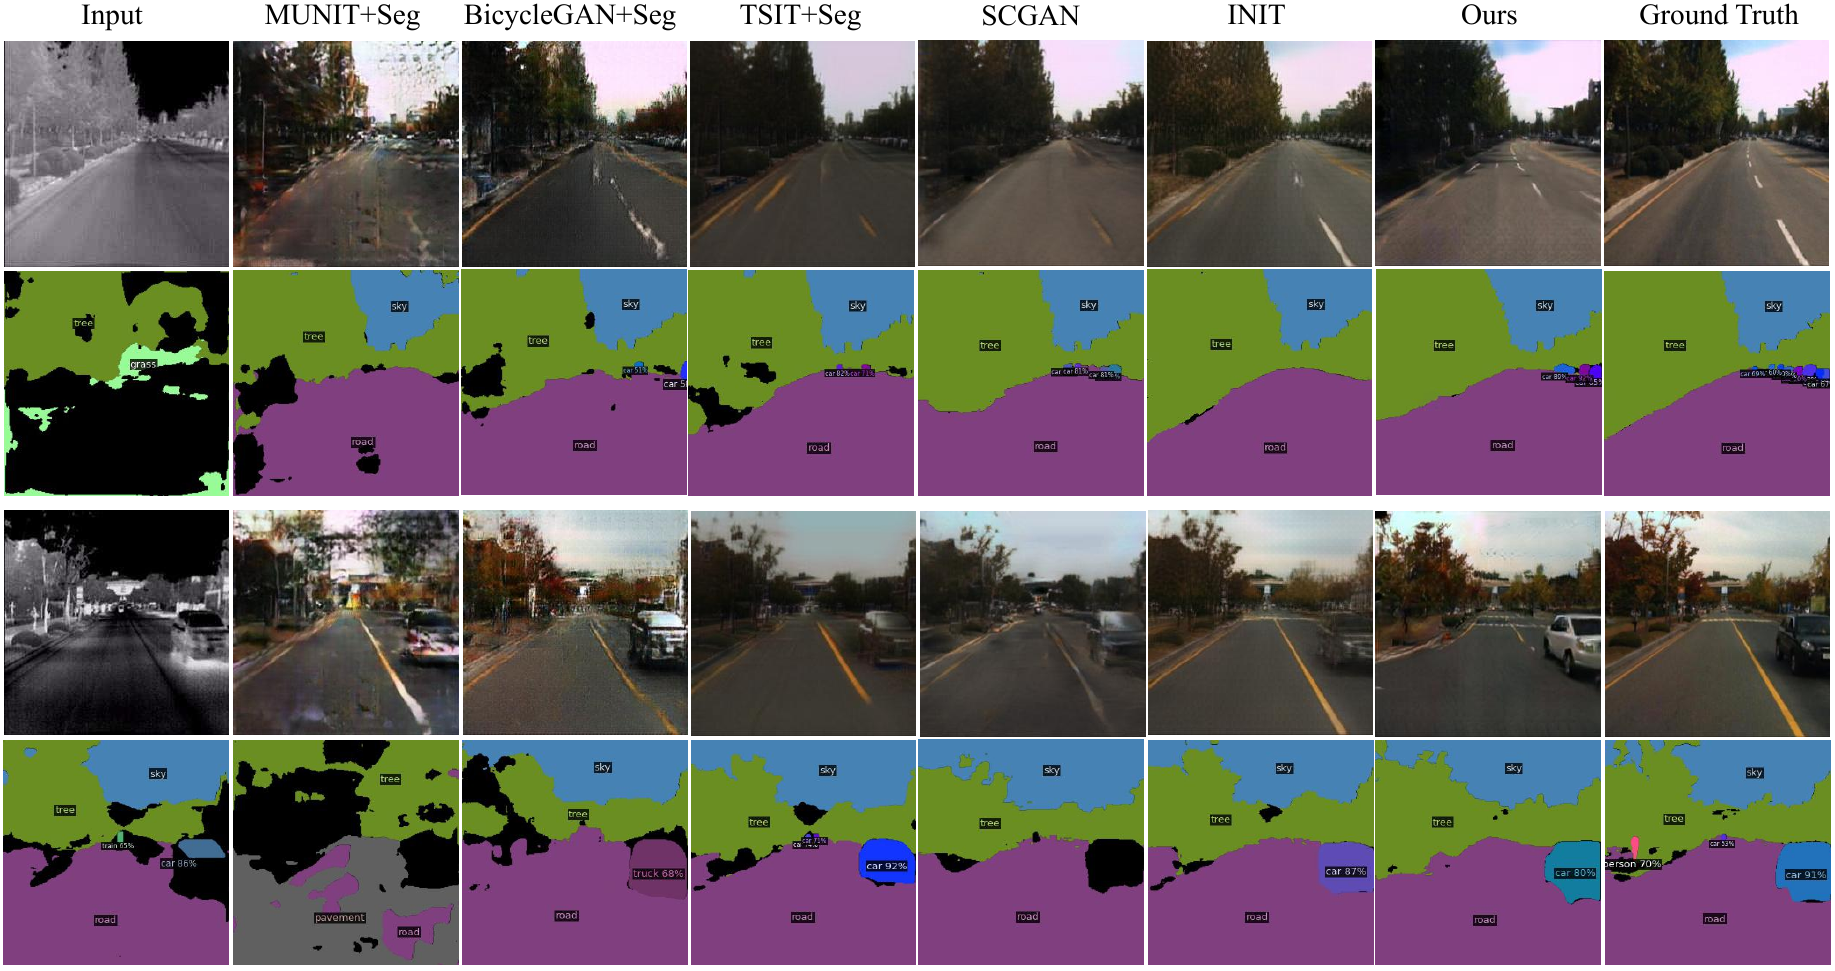}} \\
\vspace{-2.2mm}
\subfloat[{\bf The scene with multiple discrepant objects}]{
\includegraphics[width=1.0\linewidth]{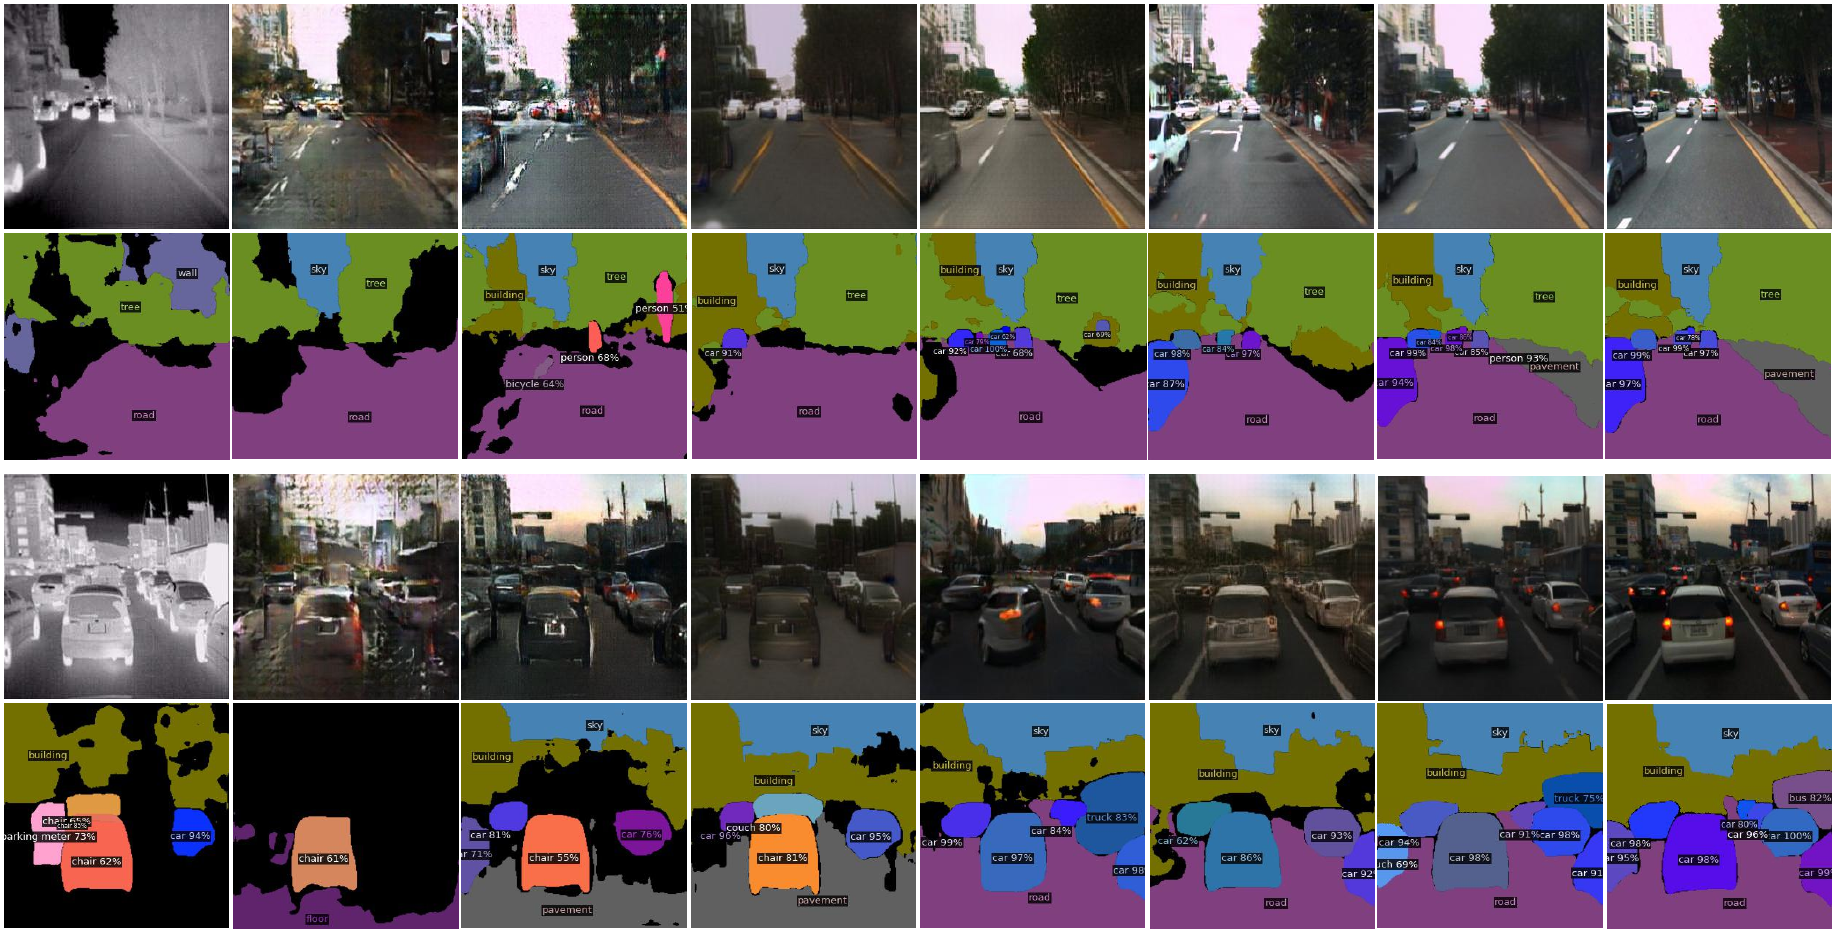}} \\
\end{center}
    \caption{The object recognition performance of translated images for different approaches. Top group denotes the scene with fewer objects; Bottom group denotes the scene with multiple discrepant objects. In each group, upper row are translated images from different approaches, lower row are the results of the corresponding panoptic segmentation.}
\label{fig:perception}
\end{figure*}
%-------------------------------------------------------------------------

\section{Limitations}
\label{sec:limitations}
As we finely perceive the foreground object instances `thing' and background semantic regions `stuff' \cite{Panoptic-Segmentation} to learn the translation model.
For `thing' (\eg, car), it can generate different details for high diversity.
However, for `stuff' (\eg, road), if generated `stuff' texture is highly different from the ground truth (\eg, the road has largely different lane markings and zebra crossings), it may decrease the whole image quality to some extent and thus affect the object recognition performance as well.
This is because the `stuff' normally has a larger region than `thing', which should be considered with the majority of the whole image context.
%-------------------------------------------------------------------------

{\small
\bibliographystyle{ieee_fullname}
\bibliography{egbib}
}

\end{document}
